# Supplementary material for: AET-SGD: Asynchronous Event-triggered Stochastic Gradient Descent
Source: arXiv:2112.13935 source file (2021-12-27)
Supplement: Supplementary file 2 [file 06_Appendix_Experiment.tex]

\section{Additional Experiments}
